# Supplementary material for: AgentsCoDriver: Large Language Model Empowered Collaborative Driving with Lifelong Learning
Source: arXiv:2404.06345 source file (2024-04-21)
Supplement: Supplementary file 1 [file 06_appendix.tex]

% \section{You \emph{can} have an appendix here.}

% You can have as much text here as you want. The main body must be at most $8$ pages long.
% For the final version, one more page can be added.
% If you want, you can use an appendix like this one.  

% The $\mathtt{\backslash onecolumn}$ command above can be kept in place if you prefer a one-column appendix, or can be removed if you prefer a two-column appendix.  Apart from this possible change, the style (font size, spacing, margins, page numbering, etc.) should be kept the same as the main body.

\section{Related Work}
\label{appendix:related_work}

\subsection{Development of Large Language Models}

Recent development of Large Language Models (LLMs), such as GPT-3 \cite{brown2020language}, PaLM \cite{chowdhery2023palm}, and GPT-4 \cite{sanderson2023gpt}, has revolutionized the field of artificial intelligence (AI). These models, characterized by their immense parameter size and pre-trained on extensive datasets, have demonstrated remarkable capabilities in text generation and comprehension. A key feature distinguishing LLMs from their predecessors is their emergent abilities, such as in-context learning, instruction following, and reasoning with chain-of-thought, which are instrumental in their advanced performance \cite{wei2022chain,wang2022self,zhang2022automatic,linPushingLargeLanguage2023,lin2024efficient}. Moreover, the alignment of LLMs with human objectives, such as truthfulness and the elimination of biases, has been a focal point of research \cite{wolf2023fundamental,song2023preference}. This is crucial because biases in LLMs, reflecting those of their training data sources, can significantly impact their output \cite{blodgett2020language,sheng2021societal}. Efforts to generate opinions that find consensus across diverse groups \cite{bakker2022fine} or to design prompts to mitigate biases \cite{liu2023pre} exemplify this direction. LLMs, like ChatGPT and GPT-4, have opened avenues toward Artificial General Intelligence (AGI), showcasing human-like intelligence \cite{zhao2023survey,zhu2023minigpt}. Their application extends beyond text generation to domains like robotic tasks, such as design, navigation, and planning \cite{shah2023navigation,dorbala2023can}. The integration of LLMs in planning, particularly in dynamic, multi-agent environments, has shown promise \cite{huang2022inner}. These models can quickly understand and navigate unfamiliar environments, a task traditionally challenging for standard planning methods. This capability is particularly relevant in autonomous driving, where rapid decision-making in varying contexts is critical. 

\subsection{Large Language Models for Autonomous Driving}
In autonomous driving, significant advances in planning and decision-making have been achieved \cite{kelly2003reactive,zhang2022rethinking}. However, challenges in interpretability and data limitations remain \cite{gohel2021explainable,arrieta2020explainable,singh2023recent,atakishiyev2021explainable,lin2024adaptsfl,lin2023fedsn}. To address these, recent research has integrated LLMs into autonomous systems for enhanced reasoning and interpretability \cite{fu2024drive,chen2023driving}. However, these approaches still grapple with translating LLM reasoning into practical driving maneuvers. LLMs have shown promise in autonomous driving with their advanced cognitive and reasoning capabilities \cite{radford2018improving,radford2019language,brown2020language,ouyang2022training}. Applications of LLMs range from fine-tuning pre-trained models \cite{liu2023mtd,chen2023driving,xuDriveGPT4InterpretableEndtoend2023} to innovative prompt engineering \cite{wenDiLuKnowledgeDrivenApproach2023,cui2023receive}. Despite significant advances, challenges like inference speed and limited real-world application still persist. Additionally, LLMs have great potential to improve adaptability in perception stages in autonomous driving systems \cite{radford2021learning,mao2023language,qian2023nuscenes}. Techniques like PromptTrack \cite{wu2023language} and HiLM-D \cite{ding2023hilm} showcase LLMs' effectiveness in detection and tracking, yet real-world complexity remains a significant challenge. This paper aims to further exploit LLMs in high-level decision-making for autonomous driving, particularly in complex scenarios like navigating intersections and roundabouts, thereby advancing the field towards practical, LLM-driven collaborative driving systems.
% \subsection{Large Language Models Powered Autonomous Agents}

\subsection{Multi-Agent Collaborative Driving}

Recently, numerous works have explored the LLM-based multi-agent collaboration and communication \cite{huAdaptiveCommunicationsCollaborative2023,huFullsceneDomainGeneralization2023,hu2024collaborative,palanisamyMultiAgentConnectedAutonomous2020,shalev-shwartzSafeMultiAgentReinforcement2016}. Zhang \textit{et al.} \cite{zhangBuildingCooperativeEmbodied2023a} proposed a framework that leverages LLMs to build collaborative embodied agents, which can communicate with each other to collaboratively achieve a goal in various embodied environments. Hong \textit{et al.} \cite{hongMetaGPTMetaProgramming2023} designed MetaGPT, which is a meta-programming framework that integrates human workflows into LLM-based multi-agent collaboration. Li \textit{et al.} \cite{liCAMELCommunicativeAgents2023} developed CAMEL, a role-playing framework that allows different agents to communication with each other to facilitate autonomous collaboration. As for connected and autonomous driving, a lot of works focus on collaborative perception \cite{chenVehicleServiceVaaS2023,FangzhengruPACS}, which enhances perception by sharing data among agents. In addition, promising datasets like V2X-SIM \cite{li2022v2x}, OPV2V \cite{xu2022opv2v}, and DAIR-V2X  \cite{yu2022dair} were collected for this purpose.  F-Cooper \cite{chen2019f} and V2VNet \cite{wang2020v2vnet} leveraged specific features or graph neural networks to perform more efficient data integration. Some latest methods like DiscoNet \cite{mehr2019disconet} and Where2comm \cite{hu2022where2comm} optimized communications and took advantage of early or intermediate fusion. However, in this paper, we focus on leveraging LLMs to enable end-to-end collaborative decision-making for collaborative driving.

\section{Additional Details of \textsc{AgentsCoDriver}}\label{sec:additional_details_agentscodriver}

\subsection{Scenario Description}\label{appdx:scenario_description}
Since we leverage GPT-3.5-turbo as our foundational model, which is a single-modal model that can just process texts, so we need to encode the scenario to text that LLM can understand. In order to achieve this goal, we first extract the necessary information from the simulation environment, including each vehicle's coordinate $(x, y)$, velocity $(v_x, v_y)$, and the trigonometric headings $(\cos\theta, \sin\theta)$. Then, we use these raw data to generate a description of the scenario. Examples are shown as follows.

\begin{tcolorbox}
    [colback=gray!20, colframe=gray!100, sharp corners, leftrule={3pt}, rightrule={0pt}, toprule={0pt}, bottomrule={0pt}, left={2pt}, right={2pt}, top={3pt}, bottom={3pt}]
    \textbf{Example 1} \\ \\
    \small 
    \texttt{You are driving toward the intersection. Your current speed is 8.06 meter per second and you are 25.01 meters away from the intersection.}
    \begin{itemize}
        \item \texttt{veh1 is driving in front of you, its speed is 8.22 meter per second and it is 21.79 meter away from you.}
        \item \texttt{veh1 is driving in the intersection area (less than 5 meters away), its distance from the intersection is 3.72 meters, and its speed is 8.22 meter per second.}
    \end{itemize}
\end{tcolorbox}

\begin{tcolorbox}
    [colback=gray!20, colframe=gray!100, sharp corners, leftrule={3pt}, rightrule={0pt}, toprule={0pt}, bottomrule={0pt}, left={2pt}, right={2pt}, top={3pt}, bottom={3pt}]
    \textbf{Example 2} \\ \\
    \small 
    \texttt{You are driving on a highway with five lanes and you are driving on one of the middle lanes. Your current speed is 12.02 meter per second  and lane position is 260.03 meters. These cars are around you:}
    \begin{itemize}
        \item \texttt{veh3 is driving in front of you and in the same lane, its speed is 9.97 meter per second, and lane position is 296.89 meters.}
        \item \texttt{veh2 is driving in front of you and on your left lane, its speed is 19.25 meter per second, and lane position is 293.75 meters.}
        \item \texttt{veh4 is driving in front of you and on your right lane, its speed is 10.34 meter per second, and lane position is 305.07 meters.}
    \end{itemize}
\end{tcolorbox}

\subsection{Reasoning Engine}\label{appdx:reasoning_engine}

In order to make a driving decision, we need to synthesize information received by other modules and then reason over it. Since designing a reasoning engine from scratch is an infeasible task, we leverage powerful LLMs directly as the reasoning engine, which plays an important role in the framework.

The detailed process is shown in Alg. \ref{alg:reasoning_engine}. In addition, it is important to design a portable and efficient prompt for the reasoning engine, which is the key to the success of the framework. In order to achieve this goal, we carefully design a prompt structured as shown in Fig. \ref{fig:reason_prompt}.

\begin{figure}[htbp]
    \centering
    \includegraphics[width=0.3\linewidth]{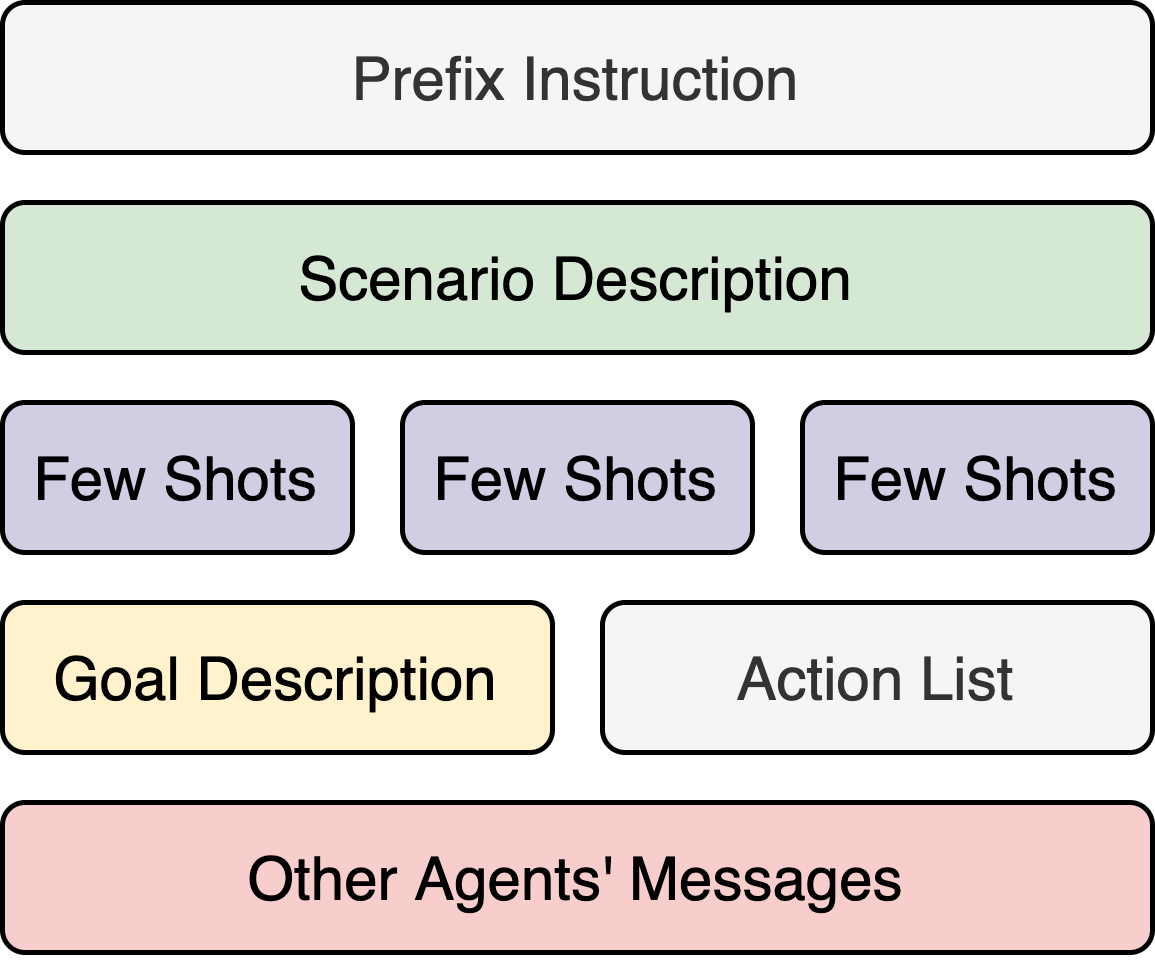}
    % \vspace{-5mm}

    \caption{Prompt design of the reasoning engine.}
    \vspace{-3mm}
    \label{fig:reason_prompt}
\end{figure}

This prompt consists of several parts: prefix instruction, scenario description, few shots, goal description, action list, and messages from other agents.

\textbf{Prefix Instruction} is a system instruction and fixed at each step, which is used to instruct the LLM how to generate the final decision. The prefix instruction is shown as follows.
\begin{tcolorbox}
    [colback=gray!20, colframe=gray!100, sharp corners, leftrule={3pt}, rightrule={0pt}, toprule={0pt}, bottomrule={0pt}, left={2pt}, right={2pt}, top={3pt}, bottom={3pt}]
    \textbf{Example Prefix Instruction} \\ \\
    \small 
    \texttt{You now should act as a skilled driver. You will be given the description of the driving scenario, available actions, some messages from other agents, some past experiences, and the goal that you need to achieve. You should follow these basic commonsense rules:}
    \begin{itemize}
        \item \texttt{You should keep your speed if your distance to the intersection is far.}
        \item \texttt{You should be slower if your distance from intersection is close.}
        \item \texttt{If there is no vehicle around the intersection, and you are near the intersection, you should speed up and quickly pass the intersection.}
    \end{itemize}

    \texttt{Your should think step by step and the response should use the following format:}
    \begin{itemize}[itemsep=2pt,topsep=0pt,parsep=0pt]
        \item \texttt{<Your reasoning process>}
        \item \texttt{<Your reasoning process>}
        \item \texttt{<Repeat until you have a final decision>}
    \end{itemize}

    \texttt{Once you have a final decision, you should output it in the following format:}
    
    \texttt{Final Decision: <Your final decision>, <The corresponding action id>}\\

    \texttt{The output decision must be unique and not ambiguous. For example, if you think idle is safe and you want to keep idle, you can output:}

    \texttt{Final Decision: idle, 1}

\end{tcolorbox}

\textbf{Scenario Description} is the description of the current scenario, which is generated by the scenario description module. Examples can be found in Appdx. \ref{appdx:scenario_description}.

\textbf{Few Shots} are the past experiences similar to the current scenario. The agent retrieves the experiences from the memory module. One shot is a memory item which consists of the scenario description, the available actions, the reasoning process, and the final decision. One example of the few shots is shown as follows. In Fig. \ref{fig:reason_prompt}, the number of shots is 3, and we can set different number of shots in each experiment.

\begin{tcolorbox}
    [colback=gray!20, colframe=gray!100, sharp corners, leftrule={3pt}, rightrule={0pt}, toprule={0pt}, bottomrule={0pt}, left={2pt}, right={2pt}, top={3pt}, bottom={3pt}]
    \textbf{Example of one shot} \\ \\
    \small 
    \texttt{\# Scenario Description}\\
    \texttt{You are going to drive across a right-angle intersection, your current speed is 10.0 m/s,  and you are 48.33 m away from the intersection.}
    \begin{itemize}
        \item \texttt{veh1 is driving behind you, its speed is -8.43 m/s,and it is 32.91 m away from you.}
        \item \texttt{veh2 is driving in front of you, its speed is 8.52 m/s, and it is 38.90 m away from you.}
        \item \texttt{veh2 is driving near the intersection (less than 10 m) and its distance from the intersection is 9.58 m.}
    \end{itemize}
    \texttt{\# Available Actions}\\
    \texttt{You can take one of the following actions: idle, accelerate, decelerate}\\

    \texttt{\# Reasoning}
    \begin{itemize}
        \item \texttt{IDLE: since my distance is not very close, I will keep my speed.}
        \item \texttt{FASTER: since I am going to approach the intersection, it is not safe to speed up.}
        \item \texttt{SLOWER: since the distance between me and the intersection is not very close, I will keep speed.}
    \end{itemize}
    \texttt{Final Decision: idle, 1}
\end{tcolorbox}
\textbf{Goal Description} is the description of the goal that the agent needs to achieve. The goal description is set manually. One of the goal descriptions is shown as follows.

\begin{tcolorbox}
    [colback=gray!20, colframe=gray!100, sharp corners, leftrule={3pt}, rightrule={0pt}, toprule={0pt}, bottomrule={0pt}, left={2pt}, right={2pt}, top={3pt}, bottom={3pt}]
    \textbf{Example of Goal Description} \\ \\
    \small 
    \texttt{Your driving goal is to drive safely and smoothly and you may communicate with other agents to collaboratively achieve this goal.}
\end{tcolorbox}

\textbf{Action List} is the list of available actions that the agent can take. The meta actions are listed in Appdx. \ref{appdx:meta_actions}.

\textbf{Messages from Other Agents } are the messages from other agents.

\begin{algorithm}[t]
    \caption{Reasoning Engine for Decision Making}
    \label{alg:reasoning_engine}
    \begin{algorithmic}[1]
    
    \Procedure{ReasoningEngine}{}
        \While{Vehicle is operational}
            \State $Prompt \gets PromptGeneration()$
            \State $Decision \gets ReasoningProcess(Prompt)$
            \State $MotionPlanning(Decision)$
        \EndWhile
    \EndProcedure
    
    \Procedure{PromptGeneration}{}
        \State Monitor surroundings to get scenario description
        \State Encode description into embeddings
        \State Retrieve Top-K related memories (experience and reflection)
        \State Combine scenario, memories, and messages into prompt
        \State \Return $Prompt$
    \EndProcedure
    
    \Procedure{ReasoningProcess}{$Prompt$}
        \State Initialize LLM with chain-of-thought technique
        \State Synthesize information from $Prompt$
        \State Reason over current state, messages, experiences, and goals, etc.
        \State Generate final decision
        \State \Return $Decision$
    \EndProcedure
    
    \Procedure{MotionPlanning}{$Decision$}
        \State Decode $Decision$ into specific actions
        \State Execute actions leading to state transition
    \EndProcedure
    
    \end{algorithmic}
    \end{algorithm}
    
\subsection{Reinforcement Reflection} \label{appdx:reinforcement_reflection}

Reflection is a critical component of the framework. The reinforcement reflection module is used to reflect on the decision made by the agent and provide feedback to the agent. Different from the traditional reinforcement learning, rewards are generated by the evaluator.
As shown in Fig. \ref{fig:iterative_reflection}, the inputs of the evaluator are scenario description, agent's reasoning process and actions, the inputs of the reflector are scenario description, agent's reasoning process and actions. The output is the reward score from the evaluator. The reflection process is shown in Alg. \ref{alg:reinforcement_reflection}.

The prompts of the evaluator consists of prefix instruction, scenario description, reasoning process, and final decision of the agent. Here we show the prefix instruction of the evaluator as follows.

\begin{tcolorbox}
    [colback=gray!20, colframe=gray!100, sharp corners, leftrule={3pt}, rightrule={0pt}, toprule={0pt}, bottomrule={0pt}, left={2pt}, right={2pt}, top={3pt}, bottom={3pt}]
    \textbf{Prefix Instruction of the Evaluator} \\ \\
    \small 
    \texttt{Now you should act like a driver's evaluator. Your duty is to evaluate the agent's decision and generate a reward score. You will be given the description of the driving scenario, the agent's reasoning process, and final decision. You should follow these basic rules: 1) If you find the agent's action is safe and reasonable, you should output CORRECT, 2) If you find the agent's action is unsafe or may cause collision, you should output INCORRECT.}
\end{tcolorbox}

The prompts of the reflector consists of prefix instruction, scenario description, reasoning process, final decision, and the output of the evaluator. The prefix instruction of the reflector is shown as follows.

\begin{tcolorbox}
    [colback=gray!20, colframe=gray!100, sharp corners, leftrule={3pt}, rightrule={0pt}, toprule={0pt}, bottomrule={0pt}, left={2pt}, right={2pt}, top={3pt}, bottom={3pt}]
    \textbf{Prefix Instruction of the Evaluator} \\ \\
    \small 
    \texttt{Now, you are a driver with rich driving skills and should reflect certain driving decisions. You will be given some information, including a description of a driving scenario, the corresponding responses (driving decisions and analysis result), and the evaluator's evaluation. You need to judge each decision and analysis logic based on the evaluation. In your final reply, provide the correct response and explain the reason for each error as well as lessons learned. Finally, give the correct answer just like the following format: <the format of the output>}
\end{tcolorbox}

\begin{algorithm}[t]
    \caption{Reinforcement Reflection Algorithm}
    \label{alg:reinforcement_reflection}
    \begin{algorithmic}[1]
        \Procedure{ReinforcementReflection}{$AgentAction, EnvObservation, AgentReasing$}
    \State $RewardScore \gets Evaluator(AgentAction, AgentReasoning, EnvObservation)$
    \State $Feedback \gets Reflector(RewardScore, AgentAction, AgentReasoning, EnvObservation)$
    \State Store $Feedback$ in $AgentMemory$
\EndProcedure

\Procedure{Evaluator}{$AgentAction, AgentReasoning, EnvObservation)$}
    \State Initialize LLM as Evaluator
    \State Generate Reward Score based on $AgentOutput$ and $EnvObservation$
    \State \Return $RewardScore$
\EndProcedure

\Procedure{Reflector}{$RewardScore, AgentAction, AgentReasoning, EnvObservation$}
    \State Initialize LLM as Reflector
    \State Detail reasons for incorrect actions
    \State Suggest improvements
    \State Provide the lessons learned
    \State \Return $Feedback$
\EndProcedure

    \end{algorithmic}
\end{algorithm}

\subsection{Communication Module} \label{appdx:communication_module}

It is vital for collaborative agents to communicate with each other effectively. By communicating with each other, the observation range of the agent will be expanded. Consider two agents' observation are $o_1$ and $o_2$, respectively. If the two agents exchange the observation information with each other, then the observation of the two agents will be expanded to $o_1 \cup  o_2$. In addition, the communication is also vital for the agents to negotiate with each other and make a better decision. For example, if an agent is driving a car, wants to overtake the front vehicle, and the agent communicates with the front vehicle, then the agent of the front vehicle can know the intention of the vehicle behind  and the agent of the front vehicle can make better decisions.

In order to realize effective communications, it is important to figure out when to communicate and what to communicate for. In order to achieve these goals, we directly leverage the agent itself to determine whether to communicate at each step and instantiate another LLM as the message generator to determine what to communicate for.
In order to deal with this issue, we instantiate an LLM as the message generator. We integrate this generator as a tool that the agent can use. When the agent think it is necessary to communicate with others, it will call this tool and feed the current encoded scenario, the messages from the other agents (if any), the previous action into the message generator, and then generate the messages to communicate with other agents. In order to facilitate the communications, we design a structured message template, which consists of \textit{prefix instruction, action history, dialogue history,} and \textit{scenario description.} 

\textbf{Prefix Instruction} is a system instruction and fixed at each step, which is used to instruct the LLM how to generate the messages. The prefix instruction is shown as follows.

\begin{tcolorbox}
    [colback=gray!20, colframe=gray!100, sharp corners, leftrule={3pt}, rightrule={0pt}, toprule={0pt}, bottomrule={0pt}, left={2pt}, right={2pt}, top={3pt}, bottom={3pt}]
    \textbf{Example of Prefix Instruction of Communication Module} \\ \\
    \small
    \texttt{You now should act like a driver's communicator. Your duty is to generate appropriate messages to communicate with other agents. You will be given the description of the driving scenario, the action history, the dialogue history, and the goal that you need to achieve.}
\end{tcolorbox}

% \textbf{Goal Description.} The goal of the communication module is not same as the agent's goal. The example is shown as follows.
% \begin{tcolorbox}
%     [colback=gray!20, colframe=gray!100, sharp corners, leftrule={3pt}, rightrule={0pt}, toprule={0pt}, bottomrule={0pt}, left={2pt}, right={2pt}, top={3pt}, bottom={3pt}]
%     \textbf{Example of Goal Description} \\ \\
%     \small 
%     \texttt{Your communication goal is to communicate with other agents to achieve the driving goal.}
% \end{tcolorbox}

\textbf{Action History} is the $N$ historical actions of the agent.

\textbf{Dialogue History} is the $M$ historical messages between the agents.

\textbf{Scenario Description} is the description of the current scenario, which is generated by the scenario description module. Examples can be found in Appdx. \ref{appdx:scenario_description}.

\section{Additional Details of the Simulation Environment and Experiments}

\subsection{Meta Actions}\label{appdx:meta_actions}

In order to control a vehicle, HighwayEnv provides five meta actions, which are listed below. The vehicle can only take one action at each time step. The action space is discrete.
\begin{itemize}[itemsep=2pt,topsep=0pt,parsep=0pt]
    \item \texttt{IDLE}: Keep the current speed and the current lane.
    \item \texttt{LANE\_LEFT}: Change lane to the left of the current lane.
    \item \texttt{LANE\_RIGHT}: Change lane to the right of the current lane.
    \item \texttt{ACCELERATE}: Accelerate the vehicle.
    \item \texttt{DECELERATE}: Decelerate the vehicle.
\end{itemize}

\begin{figure}[t]
    \centering
    % \vspace{-3mm}
    \subfigure[Multi-Vehicle Setting Scenario]{
        \includegraphics[width=0.4\textwidth]{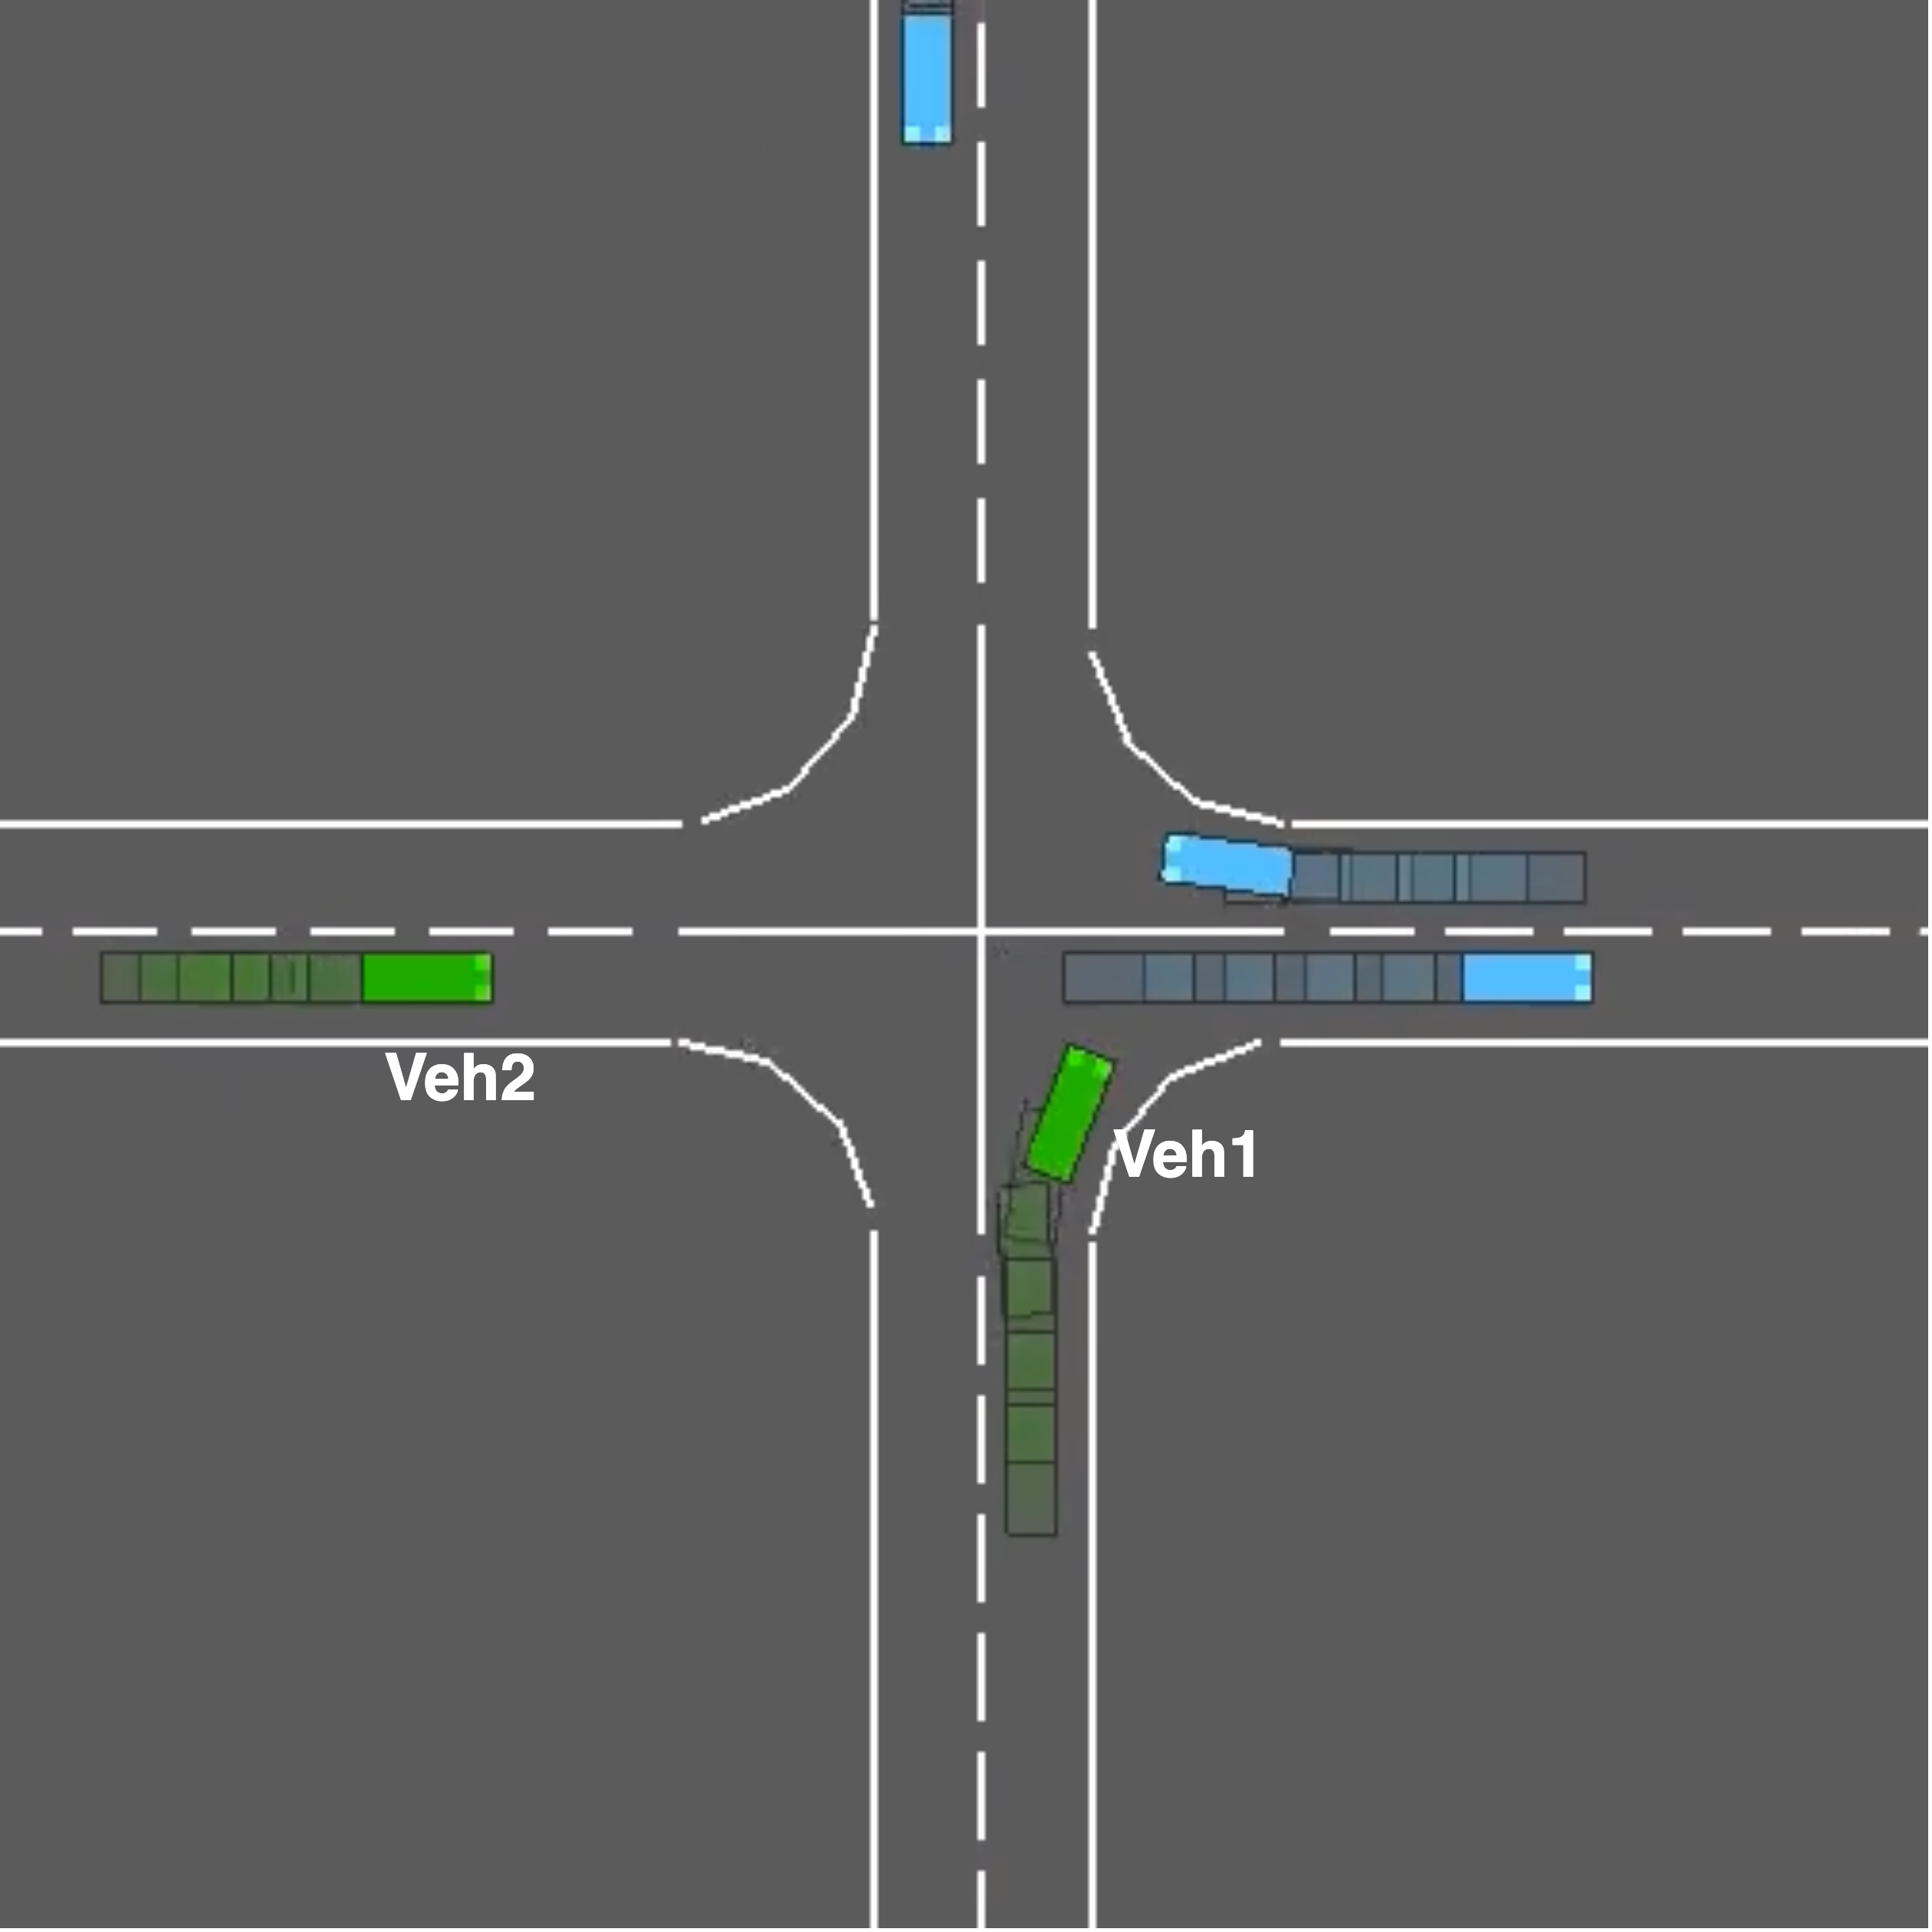}
        \label{fig:multi_vehicle_settin}
    }
    \subfigure[Single-Vehicle Setting Scenario]{
        \includegraphics[width=0.4\textwidth]{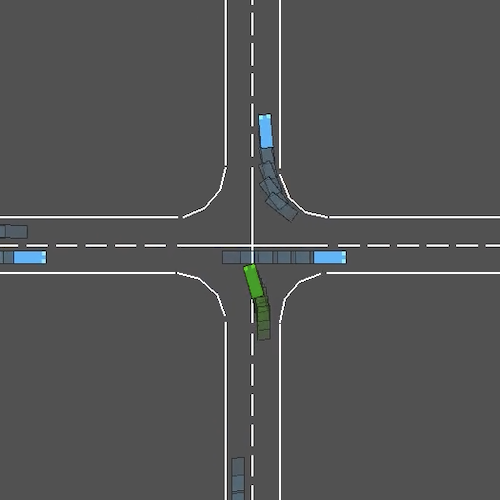}
        \label{fig:single_vehicle_setting}
    }
    \caption{Two Settings of Case Study}
\end{figure}

\subsection{Case Study}\label{appdx:case_study}

In this section, we provide some case studies of the framework to further understand how the framework works. 

\textbf{Multi-Vehicle Setting}. As shown in Fig. \ref{fig:multi_vehicle_settin}, two ego vehicles are going to cross an intersection. Veh1 is turning right and Veh2 is going straight. The two vehicles make decisions not only based on their own observations, but also based on the messages from the other vehicle. Here we show the Veh2's reasoning process and the final decision.
\begin{tcolorbox}
    [colback=gray!20, colframe=gray!100, sharp corners, leftrule={3pt}, rightrule={0pt}, toprule={0pt}, bottomrule={0pt}, left={2pt}, right={2pt}, top={3pt}, bottom={3pt}]
    \textbf{Multi-Vehicle Reasoning and Decision (examplified by \texttt{Veh2})} \\
    \small

    \texttt{\textbf{Veh1's message}: Veh2, I am turning right, my speed is 2.03 m/s, and we should keep a safe distance to avoid collision.}\\

    \texttt{\bfseries Veh2's reasoning process and decision:}
    \begin{itemize}
        \item \texttt{My position and speed: I am 21.67 m away from the center of the intersection and my current speed is 7.34 m/s.}
        \item \texttt{Intersection condition: Veh1 is in the intersection area and the intersection are is not clear. In addition, my distance to the intersection is not very close and so I can keep my speed.}
        \item \texttt{Message from the other vehicle: Veh1 said that it is  turning right, its speed is 2.03 m/s, and I should keep a safe distance to avoid collision.}
    \end{itemize}
    \texttt{I am going to approach the intersection, Veh1 is in the interaction area and turning right, and I should decelerate to keep a safe distance with it. Final Decision: decelerate, 2}\\

    \texttt{\textbf{Veh2's message}: Veh1, since you are turning right and in the intersection area, I will decelerate to keep a safe distance with you.}
\end{tcolorbox}

\textbf{Single-Vehicle Setting}. In this setting, as shown in Fig. \ref{fig:single_vehicle_setting}, an ego vehicle is going to cross an intersection, and turn left. We show the reasoning process and the final decision. 

\begin{tcolorbox}
    [colback=gray!20, colframe=gray!100, sharp corners, leftrule={3pt}, rightrule={0pt}, toprule={0pt}, bottomrule={0pt}, left={2pt}, right={2pt}, top={3pt}, bottom={3pt}]
    \textbf{Single-Vehicle Reasoning and Decision} 
    \small
    \begin{itemize}
        \item \texttt{My position and speed: I am 2.98 meters away from the center of the intersection, which means I am in the intersection area, and my current speed is 3.12 m/s.}
        \item \texttt{Intersection Condition: There is no vehicle in the intersection area and I should accelerate to pass the intersection quickly, not to block the traffic. This is an important condition to ensure that accelerating is safe and does not pose a risk to other road users.}
    \end{itemize}
    \texttt{Since the scenario indicates that I am in the intersection area, it is clear, and the decision to accelerate will help me pass the interaction. This action will help me clear the intersection more efficiently, reducing the time spent in a potentially vulnerable position. Final Decision: accelerate, 3}
\end{tcolorbox}
